# Supplementary material for: Incorporating Sum Constraints into Multitask Gaussian Processes
Source: arXiv:2202.01793 source file (2023-02-01)
Supplement: Supplementary file 1 [file SC_supplementary.pdf]

---

# Incorporating sum constraints into multitask Gaussian processes

## Supplementary material

---

Anonymous Author(s)

Affiliation

Address

email

### 1 A Free fall

2 In addition to the harmonic oscillator (see Section 4.1), we investigated the simple example of a mass  
3 in free fall as a second toy problem. Here, the output of the GP consists in position and velocity of the  
4 mass,  $\mathbf{f}^\top = [z, v]$ , whereas the time  $t$  serves as input. Then the constraint takes the following form

$$\mathcal{F}[\mathbf{f}(\mathbf{x})] = mgz(t) + m\frac{v(t)^2}{2} = E_{\text{pot}} + E_{\text{kin}} = E. \quad (\text{A.1})$$

5 In terms of (6), we identify  $a_1 = mg$ ,  $a_2 = m/2$ ,  $h_1(z) = z$ ,  $h_2(v) = v^2$  and  $C = E$ . Hence,  
6 we receive for the transformed outputs  $f'_1 = f_1 = z$  and  $f'_2 = v^2$ . We choose the auxiliary  
7 output as  $f'_3 = v$ , which we use to extract the sign when backtransforming  $f'_2$  and to create virtual  
8 measurements for  $f'_2$  at the zero crossings of  $f'_3$ . In order to fit the transformed outputs of the GP,  
9 the observations  $\mathbf{y}_k = [z_k, v_k]^\top$  are transformed analogously to obtain  $\mathbf{y}'_k = [z_k, v_k^2, v_k]^\top$ ; the virtual  
10 measurements are also included in the transformed data  $\mathbf{y}'$ . In terms of the transformed outputs the  
11 constraint can be written compactly as  $\mathbf{F}\mathbf{f}' = C$ , where  $\mathbf{F} = [a_1, a_2, 0]$ .

12 As can be seen in the left plot of Figure 4, the constrained GP yields good results for noisy data and  
13 performs better than the unconstrained GP. In the middle plot the transformed outputs are displayed  
14 together with the auxiliary outputs. In the plot on the right, we demonstrate that the constrained GP  
15 can deal better with incomplete measurements than the unconstrained one.

16 In Table 3, values for both the root mean squared error (RMSE) and the average absolute violation  
17 of the constraint  $|\Delta C|$  are given for various noise levels  $\sigma_n$  and both for the cases of complete  
18 and incomplete measurements. In case of incomplete measurements, output components have been  
19 omitted at random with probability  $f_d = 0.3$ . The values have been obtained by averaging over 50  
20 datasets. The constrained GP performs better on average, where the advantage is bigger in case of  
21 more noise.

### 22 B Background on GP regression

23 In this section we give a very brief overview of some important GP regression formulas. For more  
24 detailed accounts see e.g. [1, 27]. Given the mean function  $m(\cdot)$  and kernel  $K(\cdot, \cdot)$  of the GP, the  
25 predictive distribution of the GP can be calculated by first constructing the joint distribution between

|             |              | GP-constrained, GP-unconstrained |                        |                        |
|-------------|--------------|----------------------------------|------------------------|------------------------|
|             |              | $\sigma_n = 0.05$                | $\sigma_n = 0.1$       | $\sigma_n = 0.3$       |
| $f_d = 0$   | RMSE         | <b>2.6e-2</b> , 2.9e-2           | <b>4.1e-2</b> , 5.6e-2 | <b>1.4e-1</b> , 1.7e-1 |
|             | $ \Delta C $ | <b>1.8e-2</b> , 3.4e-1           | <b>4.2e-3</b> , 6.2e-1 | <b>3.5e-3</b> , 1.8    |
| $f_d = 0.3$ | RMSE         | <b>3.4e-2</b> , 4.1e-2           | <b>6.2e-2</b> , 8.2e-2 | <b>2.1e-1</b> , 2.5e-1 |
|             | $ \Delta C $ | <b>2.3e-2</b> , 4.9e-1           | <b>4.4e-3</b> , 8.7e-1 | <b>1.2e-2</b> , 2.5    |

Table 3: Comparison of the performance of the constrained GP and the unconstrained GP for the free fall. Shown are the root mean squared error (RMSE) of the prediction as well as the mean absolute violation of the constraint,  $|\Delta C|$ . The standard deviation of the noise is given by  $\sigma_n$  whereas  $f_d$  is the probability with which output components have been omitted at random from the data. Each of the three columns contains the results obtained for both the constrained GP and the unconstrained GP. The values have been obtained by averaging over 50 datasets. Bold font highlights best performance.

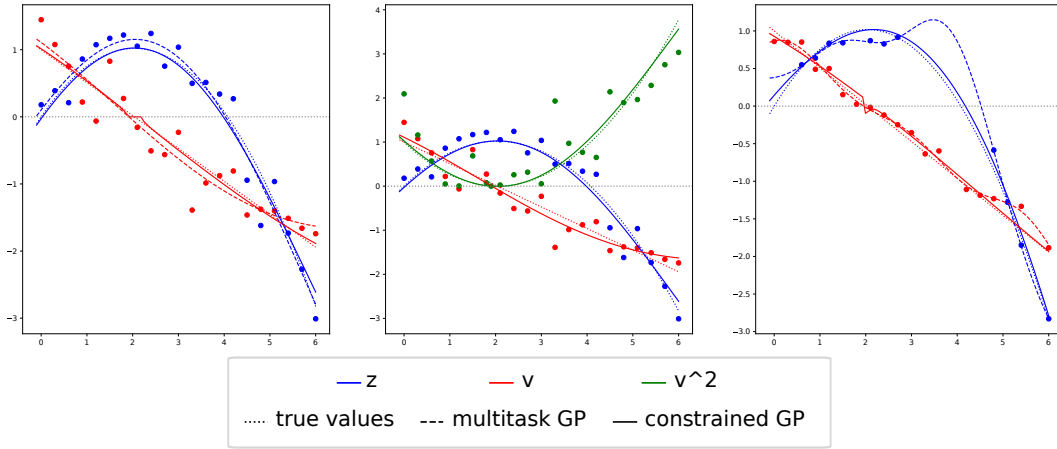

Figure 4: **Left and middle:** Demonstration of the auxiliary variables approach for the free fall. On the left the actual outputs are shown whereas in the middle plot the transformed outputs learned by the constrained GP are depicted. The outputs of the constrained GP manage to fulfill the constraint with about two orders of magnitude higher accuracy than the unconstrained GP. We observe that the constrained GP can deal better with the influence of noise than the unconstrained GP. **Right:** We consider the case of incomplete measurements. The constrained GP manages to fill in the blanks significantly better than the unconstrained one.

26 observations  $\mathbf{y}$  and function values at test locations  $\mathbf{f}_*$ ,

$$\begin{bmatrix} \mathbf{y} \\ \mathbf{f}_* \end{bmatrix} \sim \mathcal{N} \left( \begin{bmatrix} m(\mathbf{X}) \\ m(\mathbf{X}_*) \end{bmatrix}, \begin{bmatrix} K(\mathbf{X}, \mathbf{X}) + \sigma_n^2 \mathbf{I} & K(\mathbf{X}, \mathbf{X}_*) \\ K(\mathbf{X}_*, \mathbf{X}) & K(\mathbf{X}_*, \mathbf{X}_*) \end{bmatrix} \right). \quad (\text{B.1})$$

27 Then, the conditional distribution  $\mathbf{f}_* | \mathbf{X}, \mathbf{y}, \mathbf{X}_*$  is constructed as follows:

$$\mathbf{f}_* | \mathbf{X}, \mathbf{y}, \mathbf{X}_* \sim \mathcal{N}(\bar{\mathbf{f}}_*, \text{cov}(\mathbf{f}_*)), \text{ where} \quad (\text{B.2a})$$

$$\begin{aligned} \bar{\mathbf{f}}_* &\triangleq \mathbb{E}[\mathbf{f}_* | \mathbf{X}, \mathbf{y}, \mathbf{X}_*] \\ &= m(\mathbf{X}_*) + K(\mathbf{X}_*, \mathbf{X})[K(\mathbf{X}, \mathbf{X}) + \sigma_n^2 \mathbf{I}]^{-1}(\mathbf{y} - m(\mathbf{X})), \end{aligned} \quad (\text{B.2b})$$

$$\text{cov}(\mathbf{f}_*) = K(\mathbf{X}_*, \mathbf{X}_*) - K(\mathbf{X}_*, \mathbf{X})[K(\mathbf{X}, \mathbf{X}) + \sigma_n^2 \mathbf{I}]^{-1}K(\mathbf{X}, \mathbf{X}_*). \quad (\text{B.2c})$$

28 The log-marginal likelihood, which is used for hyperparameter optimization, is given by

$$\log p(\mathbf{y} | \mathbf{X}) = -\frac{1}{2}(\mathbf{y} - m(\mathbf{X}))^\top (\mathbf{K} + \sigma_n^2 \mathbf{I})^{-1}(\mathbf{y} - m(\mathbf{X})) - \frac{1}{2} \log |\mathbf{K} + \sigma_n^2 \mathbf{I}| - \frac{n}{2} \log 2\pi, \quad (\text{B.3})$$

29 where  $\mathbf{K} = K(\mathbf{X}, \mathbf{X})$ .

---

**Algorithm 2:** Constraining the GP - special case of constant task interdependencies

---

**Input:** data mean  $m_d(\cdot)$ ; data kernel  $k_d(\cdot, \cdot)$ ; task mean  $\mathbf{m}_t$ ; task covariance matrix  $\Sigma_t$ ; constraints  $(\mathbf{F}, \mathbf{S})$ ; (transformed) data  $\mathbf{X}, \mathbf{y}'$ ; points of prediction  $\mathbf{X}_*$

**Output:** constrained predictive distribution  $\mathbf{f}'_* | \mathbf{X}, \mathbf{y}', \mathbf{X}_*$

**Note:** During hyperparameter optimization  $\mathbf{X}_* = \{\}$  and hence  $\mathbf{f}'_* = \{\}$

**Step 1:** Calculate constrained  $\mathbf{m}'_t, \Sigma'_t$  according to (12b)-(12e)

**Step 2:** Construct parameters  $\mu, \Sigma$  of the (single task) joint prior distribution according to (B.1)  
-omit noise term  $\sigma_n^2 \mathbf{I}$

**Step 3:** Construct constrained (multi task)  $\mu', \Sigma'$  according to (4)

**if Hyperparameter optimization then**

**Step 4:** Calculate the log marginal likelihood according to (B.3)  
    -do not omit noise term  $\sigma_n^2 \mathbf{I}$ ; substitute corresponding blocks from  $\mu', \Sigma'$

**Step 5:** Perform optimization step

**else if Prediction then**

**Step 4:** Calculate the predictive distribution  $\mathbf{f}'_* | \mathbf{X}, \mathbf{y}', \mathbf{X}_*$  according to (B.2)  
    -do not omit noise term  $\sigma_n^2 \mathbf{I}$ ; substitute corresponding blocks from  $\mu', \Sigma'$

**end**

---

## 30 C Special case of constant constraints

31 In the special case where all of the constraints are constant and where the kernel of the GP factorizes  
32 into data and task kernel as in (4), the procedure described in Section 3.2 simplifies. It then suffices  
33 to enforce the constraints  $\mathbf{F}$  on the task mean and covariance matrix and subsequently perform the  
34 Kronecker product with the data mean and covariance matrix to obtain the constrained distribution.

35 Formally, this can be written as follows: let  $\mathbf{m}_t$  and  $\Sigma_t$  be the task mean and covariance matrix,  
36 respectively; then the constrained quantities  $\mathbf{m}'_t$  and  $\Sigma'_t$  are calculated via equations (12b)-(12e).  
37 Finally, the full constrained mean and covariance matrix are constructed via  $\mu' = \mathbf{m}_d \otimes \mathbf{m}'_t$  and  
38  $\Sigma' = \Sigma_d \otimes \Sigma'_t$ , where  $\mathbf{m}_d$  and  $\Sigma_d$  are the data mean and covariance matrix, respectively. This  
39 procedure is summarized in Algorithm 2.

40 Whenever applicable, it is preferable to use this way of incorporating the constraint as it is numerically  
41 more stable than the general procedure summarized in Algorithm 1. For the examples considered in  
42 the paper, we used this approach.

## 43 D Double pendulum parameters

44 In Section 4.3 we demonstrated the applicability of our approach to the ‘Double Pendulum Chaotic’  
45 dataset. A description of the dataset can be found in [9]; to prevent confusion, we should mention  
46 that the blue and the green marker in our paper correspond to the green and the blue marker in [9],  
47 respectively (i.e. the colors have been exchanged). The lengths of the two pendula are given as  
48  $l_b = 91$  mm and  $l_g = 70$  mm, where the suffix  $b$  refers to the pendulum with blue marker and  $g$  to the  
49 one with green marker. However, in order to calculate the energy (up to a constant factor), knowledge  
50 of the masses, or at least of the ratio  $m_b/m_g$  is required. From information given by the authors of  
51 the paper and the manufacturer of the double pendulum, together with some experimentation of our  
52 own we estimated this ratio as  $m_b/m_g \approx 6.5$ . Note that in our description of the double pendulum  
53 (14), we made the assumption that it consists of two point masses, which is only approximately true.

54 Another quantity of interest is the frame rate of the camera that was used to create the dataset; it enters  
55 into the model when calculating the velocities of the masses. In their paper [9], the authors state a  
56 frame rate of 400 Hz. However, our experiments with the dataset and keeping the energy constraint in  
57 mind strongly indicate a frame rate of 500 Hz; for 400 Hz there are segments of the motion where the  
58 total energy  $E$  clearly increases which violates the principle of energy conservation (see Figure 5).

59 The ‘Double Pendulum Chaotic’ dataset was published under the “Community Data License Agree-  
60 ment - Sharing - Version 1.0”.

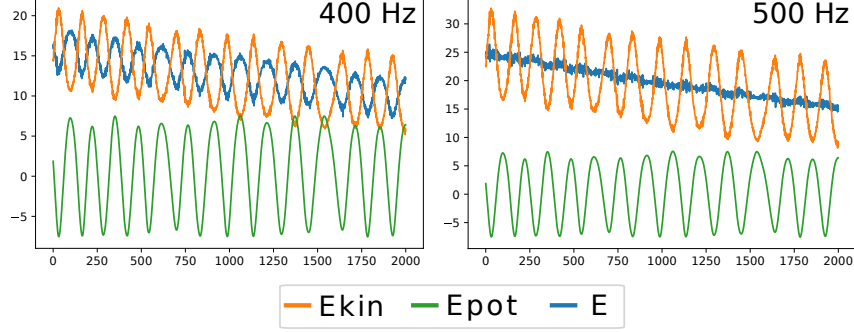

Figure 5: Comparison of the energy of the double pendulum for different frame rates of the camera. It is apparent that a frame rate of 400 Hz is incompatible with the principle of energy conservation; while the energy is decreasing in the long term due to friction, it should never increase. No choice of mass ratio  $m_b/m_g$  was able to resolve this issue. On the other hand, a frame rate of 500 Hz together with the mass ratio  $m_b/m_g = 6.5$  is compatible with energy conservation, within the bounds of error.

## 61 E Implementation details

### 62 E.1 Kernel and mean

63 Throughout the paper we use a radial basis function (RBF) kernel (also: squared exponential kernel)  
64 as data kernel,

$$k_{\text{RBF}}(\mathbf{x}, \mathbf{x}') = \sigma_f^2 \exp\left(-\frac{\|\mathbf{x} - \mathbf{x}'\|^2}{2l^2}\right), \quad (\text{E.1})$$

65 where  $\sigma_f$  is a scale factor and  $l$  is the length scale. We use the position independent index kernel  
66 provided by gpytorch [29],

$$\mathbf{k}_t = \mathbf{B}\mathbf{B}^\top + \text{diag}(\mathbf{v}), \quad (\text{E.2})$$

67 where  $\mathbf{B}$  is a low-rank matrix and  $\mathbf{v}$  is a non-negative vector; we chose the rank of  $\mathbf{B}$  to be equal to  
68 the number of tasks of the GP in question. The parameters  $\sigma_f$ ,  $l$ ,  $\mathbf{B}$  and  $\mathbf{v}$  are to be learned during  
69 the training process. For more examples of possible kernels see e.g. [1, 28]. The complete kernel is  
70 then constructed via the Kronecker product

$$\mathbf{K}_{\mathbf{f}, \mathbf{f}'}(\mathbf{X}, \mathbf{X}') = k_{\text{RBF}}(\mathbf{X}, \mathbf{X}') \otimes \mathbf{k}_t. \quad (\text{E.3})$$

71 We chose constant mean functions for all outputs of the multitask GP. All the models have been  
72 implemented in python with the library gpytorch [29].

### 73 E.2 Harmonic oscillator

74 The data for the harmonic oscillator toy problem was generated from

$$x(t) = x_0 \sin(\omega_0 t), \quad (\text{E.4a})$$

$$v(t) = x_0 \omega_0 \cos(\omega_0 t). \quad (\text{E.4b})$$

75 The energy is given by

$$E = \frac{k}{2}x^2 + \frac{m}{2}v^2 = \frac{k}{2}x_0^2 \sin^2(\omega_0 t) + \frac{m}{2}x_0^2 \omega_0^2 \cos^2(\omega_0 t). \quad (\text{E.5})$$

76 We have chosen  $E = 0.8 \text{ J}$ ,  $m = 1 \text{ kg}$ ,  $\omega_0 = 1 \text{ s}^{-1}$  and it holds that  $k = m\omega_0^2$  and  $x_0 = \sqrt{2E/k}$ .

77 Training data has been generated by evaluating the function on the equally spaced grid  $t \in$   
78  $\text{linspace}(0, 10, 20) \text{ [s]}$ . Subsequently, random noise  $\epsilon \sim \mathcal{N}(0, \sigma_n^2)$  was added to the data; the values for  
79  $\sigma_n$  are given in the main text. Test data has been generated on the grid  $t \in \text{linspace}(-0.1, 10, 100) \text{ [s]}$ .

### 80 E.3 Triangle in the plane

81 In terms of the parameter  $\alpha$ , the trajectory that we used for the triangle in the plane in Section 4.2 is  
 82 given by

$$\mathbf{Z}_0 = \begin{bmatrix} 4 & 8 & 8.4 \\ 4 & 4 & 6 \end{bmatrix}, \quad (\text{E.6a})$$

$$\mathbf{Z}_1 = \mathbf{Z}_0 + d(\alpha), \quad (\text{E.6b})$$

$$\mathbf{Z} = \mathbf{R}(\alpha)\mathbf{Z}_1 + d(\alpha), \quad (\text{E.6c})$$

83 where  $d(\alpha) = \frac{1}{2} \cos(2\alpha)$  and where  $\mathbf{R}$  is a rotation matrix. We then added an auxiliary point of  
 84 known position to each datapoint:

$$\mathbf{Z} = \begin{bmatrix} z_{1x} & z_{2x} & z_{3x} & 4 \\ z_{1y} & z_{2y} & z_{3y} & 4 \end{bmatrix}. \quad (\text{E.7})$$

85 Following the approach from [8], we constructed the matrix  $\mathbf{Q} = \mathbf{Z}^\top \mathbf{Z}$  and used the upper triangular  
 86 elements of  $\mathbf{Q}$  as outputs for the constrained GP:

$$\mathbf{y}' = [Q_{11}, Q_{12}, Q_{13}, Q_{14}, Q_{22}, Q_{23}, Q_{24}, Q_{33}, Q_{34}, Q_{44}]. \quad (\text{E.8})$$

87 Then the matrix  $\mathbf{F}$  and the corresponding vector  $\mathbf{S}$  encoding the length constraints for all the edges of  
 88 the triangle become

$$\mathbf{F} = \begin{bmatrix} 1 & -2 & 0 & 0 & 1 & 0 & 0 & 0 & 0 & 0 \\ 1 & 0 & -2 & 0 & 0 & 0 & 0 & 1 & 0 & 0 \\ 0 & 0 & 0 & 0 & 1 & -2 & 0 & 1 & 0 & 0 \\ 0 & 0 & 0 & 0 & 0 & 0 & 0 & 0 & 0 & 1 \end{bmatrix}, \quad \mathbf{S} = \begin{bmatrix} L_{12}^2 \\ L_{13}^2 \\ L_{23}^2 \\ L_{O4}^2 \end{bmatrix}, \quad (\text{E.9})$$

89 where the last row of  $\mathbf{F}$  corresponds to the constraint on the distance between the auxiliary point and  
 90 the origin of the coordinate system.

91 After training the constrained GP, learned values  $\tilde{\mathbf{y}}'$  are rearranged into the (symmetric) matrix  $\tilde{\mathbf{Q}}$ ,  
 92 analogously to (E.8). Then the matrix  $\tilde{\mathbf{Z}}$  is recovered via a singular value decomposition (SVD) of  
 93  $\tilde{\mathbf{Q}}$ ; this decomposition is not unique and the auxiliary point comes into play: we compare the learned  
 94 point with the known position and determine the angle between them to rotate the learned coordinates  
 95 to their actual positions.

96 Training data was generated on the grid  $\alpha \in \text{linspace}(0, 5, 20)$ . Subsequently, random noise  $\epsilon \sim$   
 97  $\mathcal{N}(0, \sigma_n^2)$  was added to the data; the values for  $\sigma_n$  are given in the main text. Test data was generated  
 98 on the grid  $\alpha \in \text{linspace}(0, 5, 100)$ .

### 99 E.4 Free fall

100 The data for the free fall was generated from

$$z(t) = v_0 t - \frac{g}{2} t^2, \quad (\text{E.10a})$$

$$v(t) = v_0 - gt. \quad (\text{E.10b})$$

101 The energy is given by

$$E = mgz + \frac{m}{2} v^2. \quad (\text{E.11})$$

We have chosen  $E = 200 \text{ J}$ ,  $m = 1 \text{ kg}$  and it holds that  $v_0 = \sqrt{2E/m}$ , and the gravitational acceleration on earth is  $g = 9.81 \text{ m s}^{-2}$ . Training data has been generated by evaluating the function on the equally spaced grid  $t \in \text{linspace}(0, 6, 20) \text{ [s]}$ . Subsequently, random noise  $\epsilon \sim \mathcal{N}(0, \sigma_n^2)$  was added to the data; the values for  $\sigma_n$  are given in the main text. To ensure good visibility and learnability, we scaled the data  $\mathbf{y}$  with a factor  $a = 20$ :  $\mathbf{y} \rightarrow \mathbf{y}/a$ . Both in Figure 4 and in Table 3, the results are given in terms of the rescaled data (and noise values); the results in terms of the original scale can be obtained by multiplying with  $a$ . Test data has been generated on the grid  $t \in \text{linspace}(-0.1, 6, 100) \text{ [s]}$ .

## 110 E.5 Double Pendulum

The ‘Double Pendulum Chaotic’ dataset provides data in the form of annotated positions of the masses attached to the ends of the two pendula (together with the position of the top of the apparatus holding the pendulum which does not change and which we therefore omitted). We now have the positions as points on an equally spaced grid; in terms of the camera frame rate  $r$  the spacing between two adjacent points is given by  $1/r$ . To obtain the velocities we numerically take the gradient of the positions on the grid and we receive the data which we use for our GP,  $\mathbf{y} = [z_{bx}, z_{by}, z_{gx}, z_{gy}, v_{bx}, v_{by}, v_{gx}, v_{gy}]$ . To obtain positions and velocities with comparable absolute values, which enhances the performance of the GP and which makes the quantities easier to compare in plots, we scaled positions by a factor of 20 and velocities by a factor of  $\sqrt{10}$ .

As outlined in Section 4.3, we obtain training and test data by picking a random interval of 200 datapoints from the second half of the trajectories provided by the dataset; out of those we use 15 points as training data and the rest as test data. Note that the value  $E$  received by evaluating (14) and averaging over the training data will in general be a less accurate estimate than the value of the energy  $E_0$  received when averaging over the test data, since the average is taken over fewer points. Hence, when determining the accuracy of the constraint fulfillment, the results in Section 4.3 have been compared to  $E_0$ .

## 127 E.6 Separating the outputs

As has already been mentioned before, to include virtual measurements at zero crossings for one of the transformed outputs (see Section 3.1.2), the corresponding auxiliary output has to be learned separately once before the actual constrained GP can be trained. In that case, as long as the auxiliary output is not explicitly involved in the constraint, it can be omitted from the constrained GP.

More generally, all outputs with all zero entries in the corresponding column of  $\mathbf{U}$  do not have to be learned together with the constrained outputs but can be learned in a separate GP. While not necessary, doing this is often advantageous as it keeps the dimension of the constrained GP smaller, which can improve the performance and simplify the training procedure.

In our experiments, outputs that are not affected by the constraint have been learned using a separate GP. To illustrate, let us consider the case of the double pendulum: transformed outputs together with auxiliary outputs taken together give  $\mathbf{y}' = [z_{bx}, z_{by}, z_{gx}, z_{gy}, v_{bx}^2, v_{by}^2, v_{gx}^2, v_{gy}^2, v_{bx}, v_{by}, v_{gx}, v_{gy}]$  and the corresponding constraint is given by  $\mathbf{F} = [0, m_1 g, 0, m_2 g, m_1/2, m_1/2, m_2/2, m_2/2, 0, 0, 0, 0]$ . Hence,  $\mathbf{y}'$  is 12-dimensional but only six outputs are actually involved in the constraint; so we first learn the remaining six outputs independently from the constrained ones and include only the six with non-zero entries in  $\mathbf{F}$  in the constrained GP.

## 144 E.7 Training procedure

The models have been trained using the Adam optimizer provided by gpytorch. For each experiment, the corresponding learning rate (lr) and (if applicable) scheduler settings are given in Table 4. The scheduler multiplies the learning rate with scheduler-factor after scheduler-steps iterations. The two

different scheduler parameters given for the double pendulum correspond to the constrained and the unconstrained GP, respectively.

|                       | lr  | iterations | scheduler-steps | scheduler-factor |
|-----------------------|-----|------------|-----------------|------------------|
| Harmonic oscillator   | 0.3 | 300        | -               | -                |
| Triangle in the plane | 0.1 | 2000       | 800             | 0.2              |
| Double pendulum       | 0.1 | 2000       | 800/500         | 0.2/0.5          |
| Free fall             | 0.3 | 300        | -               | -                |

Table 4: Training parameters for the experiments.

## E.8 Computing power available for the experiments

All experiments have been conducted on a system with NVIDIA GTX 1060, 6GB GPU, Intel Core i7 7700-K @ 4.2GHz CPU and 16GB RAM. The creation of average values for one set of parameters as displayed in Tables 1-3 typically took between 15 minutes and one hour.

## References

- [1] C. E. Rasmussen, and C. K. I. Williams. Gaussian Processes for Machine Learning. MIT Press (2006).
- [2] J. Willard, X. Jia, S. Xu, M. Steinbach, and V. Kumar. Integrating Physics-based Modeling with Machine Learning: A Survey. arXiv:2003.04919 (2020).
- [3] L. Swiler, M. Gulian, A. Frankel, C. Safta, and J. Jakeman. A Survey of Constrained Gaussian Process Regression: Approaches and Implementation Challenges. arXiv:2006.09319 (2020).
- [4] E. V. Bonilla, K. Ming, A. Chai, and C. Williams. Multi-task Gaussian Process Prediction. Advances in Neural Information Processing Systems 20, pp. 153-160 (2008).
- [5] G. Skolidis, and G. Sanguinetti. Bayesian Multitask Classification with Gaussian Process Priors. IEEE Transactions on Neural Networks, Vol. 22, No. 12 (2011).
- [6] M. Perriollat, R. Hartley, and A. Bartoli. Monocular Template-based Reconstruction of Inextendible Surfaces. International Journal of Computer Vision, Vol. 95, pp. 124-137 (2011).
- [7] R. Majumdar, and S. Majumdar. On the Conditional Distribution of a Multivariate Normal given a Transformation - the Linear Case. Heliyon 5 (2019) e01136.
- [8] M. Salzmann, and R. Urtasun. Implicitly Constrained Gaussian Process Regression for Monocular Non-Rigid Pose Estimation. Advances in Neural Information Processing Systems 23, pp. 2065-2073 (2010).
- [9] A. Asseman, T. Kornuta, and A. Ozcan. Learning Beyond Simulated Physics. Neural Information Processing Systems, Modeling and Decision-making in the Spatiotemporal Domain Workshop (2018).
- [10] A. Solin, and M. Kok. Know your boundaries: Constraining Gaussian Processes by Variational Harmonic Features. Proceedings of Machine Learning Research, Vol. 89, pp. 2193–2202 (2019).
- [11] S. Da Veiga, and A. Marrel. Gaussian Process Modeling with Inequality Constraints. In Annales de la Faculté des Sciences de Toulouse, Vol. 21, pp. 529–555 (2012).
- [12] H. Maatouk, and X. Bay. Gaussian Process Emulators for Computer Experiments with Inequality Constraints. Mathematical Geosciences, Vol. 49, pp. 557–582 (2017).
- [13] C. Jidling, N. Wahlström, A. Wills, and T. B. Schön. Linearly Constrained Gaussian Processes, Advances in Neural Information Processing Systems 31, pp. 1216-1224 (2017).
- [14] M. Raissi, P. Perdikaris, and G. E. Karniadakis. Machine Learning of Linear Differential Equations using Gaussian Processes. Journal of Computational Physics, Vol. 348, pp. 683–693 (2017).
- [15] M. Raissi, P. Perdikaris, and G. E. Karniadakis. Numerical Gaussian Processes for Time-Dependent and Nonlinear Partial Differential Equations. SIAM Journal on Scientific Computing, Vol. 40(1), pp. A172–A198 (2018).
- [16] N. Wahlström, M. Kok, T. B. Schön, F. Gustafsson. Modeling Magnetic Fields using Gaussian Processes. IEEE International Conference on Acoustics, Speech and Signal Processing, pp. 3522–3526 (2013).
- [17] A. Papoulis, and S. U. Pillai. Probability, Random Variables and Stochastic Processes. McGraw-Hill Education, New York (2001).
- [18] A. Solin, M. Kok, N. Wahlström, T. B. Schön, and S. Särkkä. Modeling and Interpolation of the Ambient Magnetic Field by Gaussian Processes. IEEE Transactions on Robotics, Vol. 34 (4), pp. 1112-1127 (2018).
- [19] C. Jidling, J. Hendriks, N. Wahlström, A. Gregg, T.B. Schön, C. Wensrich, and A. Wills. Probabilistic Modelling and Reconstruction of Strain. Nuclear Instruments and Methods in Physics Research Section B: Beam Interactions with Materials and Atoms, Vol. 436, 141–155 (2018).



- 201 [20] J. N. Hendriks, C. M. Wensrich, A. Wills, V. Luzin, and A. W. T Gregg. Robust Inference of  
202 Two-Dimensional Strain Fields from Diffraction-Based Measurements. *Nuclear Instruments*  
203 *and Methods in Physics Research Section B: Beam Interactions with Materials and Atoms*, Vol.  
204 444, pp. 80–90 (2019).
- 205 [21] J. Hendriks, Alex Gregg, Chris Wensrich, and Adrian Wills. Implementation of Traction  
206 Constraints in Bragg-Edge Neutron Transmission Strain Tomography. *Strain*, Vol. 55 (5) (2019).
- 207 [22] J. N. Hendriks, C. M. Wensrich, and A. Wills. A Bayesian Approach to Triaxial Strain Tomog-  
208 raphy from High-Energy X-Ray Diffraction. *Strain*, Vol. 56 (3) (2020).
- 209 [23] A. Glielmo, P. Sollich, and A. De Vita. Accurate Interatomic Force Fields via Machine Learning  
210 with Covariant Kernels. *Physical Review B*, Vol. 95 (21) (2017).
- 211 [24] B. Haasdonk, and H. Burkhardt. Invariant Kernel Functions for Pattern Analysis and Machine  
212 Learning. *Machine Learning*, Vol. 68, pp. 35–61 (2007).
- 213 [25] S. Chmiela, H. E. Sauceda, A. Tkatchenko, and K. R. Müller. Accurate Molecular Dynamics  
214 Enabled by Efficient Physically Constrained Machine Learning Approaches. *Machine Learning*  
215 *Meets Quantum Physics*, Springer International Publishing, pp. 129–154 (2020).
- 216 [26] M. Salzmann, and R. Urtasun. Combining Discriminative and Generative Methods for 3D  
217 Deformable Surface and Articulated Pose Reconstruction. *IEEE Conference on Computer*  
218 *Vision and Pattern Recognition* (2010).
- 219 [27] A. Lindholm, N. Wahlström, F. Lindsten, and T. B. Schön. *Machine Learning - A First Course*  
220 *for Engineers and Scientists*. Cambridge University Press (2021)
- 221 [28] D. J. C. MacKay. Introduction to Gaussian Processes. In C. M. Bishop, editor, *Neural Networks*  
222 *and Machine Learning*, pp. 133-165. Springer (1998).
- 223 [29] J. R. Gardner, G. Pleiss, D. Bindel, K. Q. Weinberger, and A. G. Wilson. GPyTorch: Black-  
224 box Matrix-Matrix Gaussian Process Inference with GPU Acceleration. *Advances in Neural*  
225 *Information Processing Systems* 31, pp. 7576-7586 (2018).
